# Supplementary material for: Spontaneous breaking of time-reversal symmetry at the edges of 1T' monolayer transition metal dichalcogenides
Source: arXiv:1812.09082 source file (2019-04-26)
Supplement: Supplementary file 1 [file Supplementary.pdf]

# Spontaneous breaking of time-reversal symmetry at the edges of 1T' monolayer transition metal dichalcogenides. Supplementary Material.

Line Jelver[1,2], Thomas Olsen[2], Daniele Stradi[1], Kurt Stokbro[1], and Karsten Wedel Jacobsen*[2]

[1]Synopsys Denmark, Fruebjergvej 3, PostBox 4, DK-2100 Copenhagen, Denmark.
[2]Center for Atomic-scale Materials Design (CAMD), Technical University of Denmark, Bldg. 307, DK-2800 Lyngby, Denmark.

March 4, 2019

## A Stability of the different edges

The $y$-cut of the 1T' phase can be made 6 different ways; 2 ways terminated by the metal atom, (m), 2 ways by a single chalcogenide atom, (c), and 2 ways by a pair of calcogenide atoms (2c). The 6 cuts can be seen on Fig 1. We have compared the heat of formation of the (m) and (c) type edges of $MoS_2$ using the formula,

$$E_F = E_{MoS_2}^{nanoribbon} - nE_{MoS2}^{ML} - \mu_S(E_{H_2S} - E_{H_2}) \tag{A.1}$$

$E_{MoS_2}^{nanoribbon}$ is the total energy of the nanoribbon, $n$ is the no. of ML unit cells in the nanoribbon, and $E_{MoS2}^{ML}$ is the total energy of the infinite monolayer. $\mu_S$ is a parameter which can be varied to represent different chemical potentials for sulfur. A value of $\mu_S = 1$ corresponds to taking one sulfur atom from a $H_2S$ gas. It is zero for the (c) type edge where the nanoribbon corresponds to an integer no of ML unit cells but can be varied for the (m) type edges which is missing a sulfur atom. $E_{H_2S}$ and $E_{H_2}$ is the total energy of the two molecules which are calculated with the same method as the nanoribbon and ML but in a (10x10x10) Å cell and with a single k-point. The PBE functional without SOC was used for these calculations and the (m') and (c') nanoribbons are 50 Å long. The stability of the two types of edges can be seen on Fig 2.

## B Results for nanoribbon calculation

The nanoribbon length is converged s.t. the Hartree potential is flat in the center of the ribbon. This corresponds to a length of 88 Å. 20 Å of vacuum is added to the left and right of the ribbon. On Fig 3, we show the magnetization density. The total magnetization of the nanoribbon is $135 \times 10^{-3}$ $\mu_B$ which is about twice the magnetization of the single edge and shows that the effect is additive for the two opposite edges. The electronic bands can be seen on Fig 4.

*kwj@fysik.dtu.dk

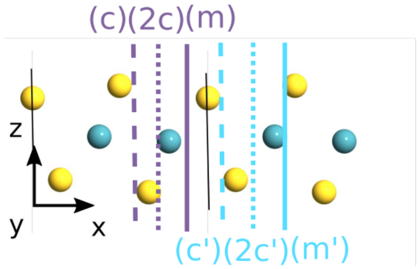


Figure 1: The six kinds of edge terminations for a cut along the y-direction.

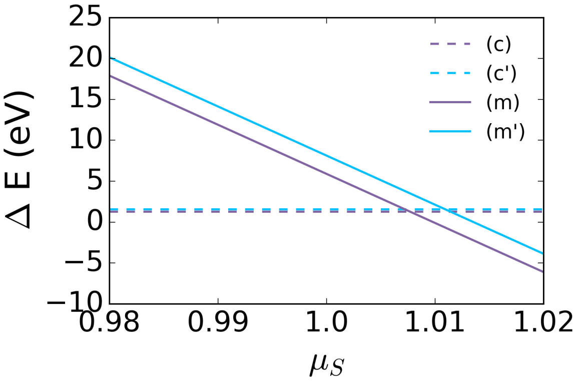


Figure 2: The stability of (m) and (c) type edges of monolayer 1T' $MoS_2$ at varying $\mu_S$.

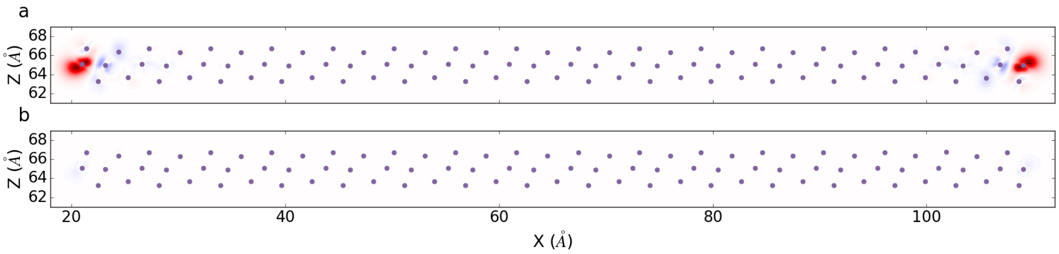


Figure 3: The magnetization density, **a** $m_x$ and **b** $m_z$ of the nanoribbon.

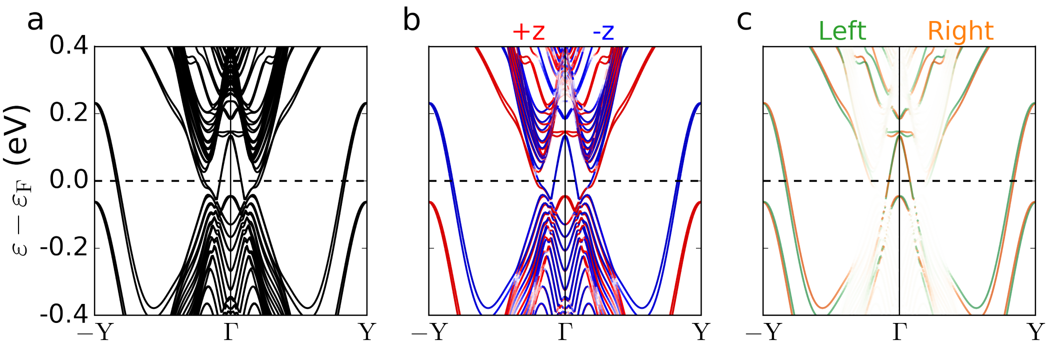


Figure 4: The electronic bands of a 1T' $MoS_2$ nanoribbon with two (m) type edges. **a** Total band structure, **b** Spin polarized band structure, and **c** projected band structure on the two edges.

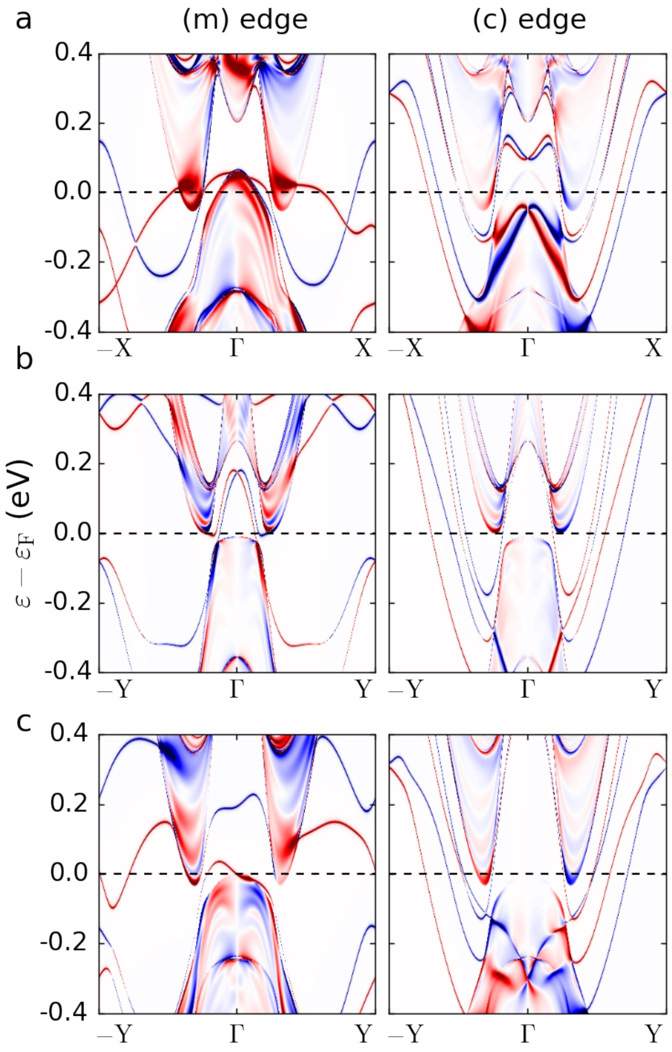


Figure 5: The electronic bands of the (m) and (c) edge of monolayer 1T' **a** $MoTe_2$, **b** $WSe_2$, and **c** $WTe_2$.

# C Results for $MoTe_2$, $WSe_2$ and $WTe_2$ edges

The electronic bands of the three TMDs can be seen on Fig 5
